# Supplementary material for: Revec: Program Rejuvenation through Revectorization
Source: arXiv:1902.02816 source file (2019-02-07)
Supplement: Supplementary file 1 [file appendix.tex]

\begin{figure}[]
\input{figures/Revec_OperationBinary8u}
\centering
\caption{A simple Pack DAG, after recursive application of \texttt{GrowDAG} is complete}
\end{figure}
